# Supplementary material for: Learning protein conformational space by enforcing physics with convolutions and latent interpolations
Source: arXiv:1910.04543 ancillary file (2020-03-25)
Supplement: Supplementary file 1 [file interp_paper_SM.pdf]

# Supplementary Material

Learning protein conformational space by enforcing  
physics with convolutions and latent interpolations

Venkata K. Ramaswamy\*

Chris G. Willcocks\*

Matteo T. Degiacomi\*

---

\*The authors contributed equally.

## 1 Evaluation of the network generated protein structures

We performed a ProSA evaluation of MurD crystal structures of open (PDB: 1E0D) and closed (PDB: 3UAG) state, as well as intermediate conformations generated by our best network. The resulting model quality scores (Z-score) were comparable (open =  $-11.01$ , closed =  $-10.62$ , interpolation =  $-11.00 \pm 0.23$ ), and fell within the range of scores typically found for native proteins of similar size. The local quality of the model based on interaction energies for each residue as evaluated with ProSA served as additional proof of model quality, with most of the residues falling in the negative energy scale and only a small subset of them on the positive side. All the observed values for our interpolated structures were within ranges also observed for the experimental structures, thereby increasing the confidence in the intermediate transition state structures generated by our neural network.

Table S 1: Convolution kernel weights

| Angle   | Atomic order    | Mask $c_1$         | Mask $c_2$         | Applicable residues |
|---------|-----------------|--------------------|--------------------|---------------------|
| N-CA-C  | N, CA, C        | [ 1, -1, 0 ]       | [ 0, -1, 1 ]       | GLY                 |
|         | N, CB, CA, C    | [ 1, 0, -1, 0 ]    | [ 0, 0, -1, 1.0 ]  | PRO                 |
|         | N, CA, CB, C    | [ 0, -1, 0, 1 ]    | [ 1, -1, 0, 0.0 ]  | Others              |
| CA-C-O  | CA, C, O        | [ 1, -1, 0 ]       | [ 0, -1, 1 ]       | GLY, PRO            |
|         | CA, CB, C, O    | [ 1, 0, -1, 0 ]    | [ 0, 0, -1, 1 ]    | Others              |
| O-C-N   | C, O, N         | [ -1, 1, 0 ]       | [ -1, 0, 1 ]       | All                 |
| N-CA-CB | N, CB, CA       | [ 0, 1, -1 ]       | [ 1, 0, -1 ]       | PRO                 |
|         | N, CA, CB       | [ 0, -1, 1 ]       | [ 1, -1, 0 ]       | Others              |
| CB-CA-C | CB, CA, C       | [ 1, -1, 0 ]       | [ 0, -1, 1 ]       | PRO                 |
|         | CA, CB, C       | [ -1, 1, 0 ]       | [ -1, 0, 1 ]       | Others              |
| CA-C-N  | CA, C, O, N     | [ 1, -1, 0, 0 ]    | [ 0, -1, 0, 1 ]    | GLY, PRO            |
|         | CA, CB, C, O, N | [ 1, 0, -1, 0, 0 ] | [ 0, 0, -1, 0, 1 ] | Others              |
| C-N-CA  | C, O, N, CB, CA | [ 0, 0, -1, 0, 1 ] | [ 1, 0, -1, 0, 0 ] | PRO                 |
|         | C, O, N, CA     | [ 0, 0, -1, 1 ]    | [ 1, 0, -1, 0 ]    | Others              |

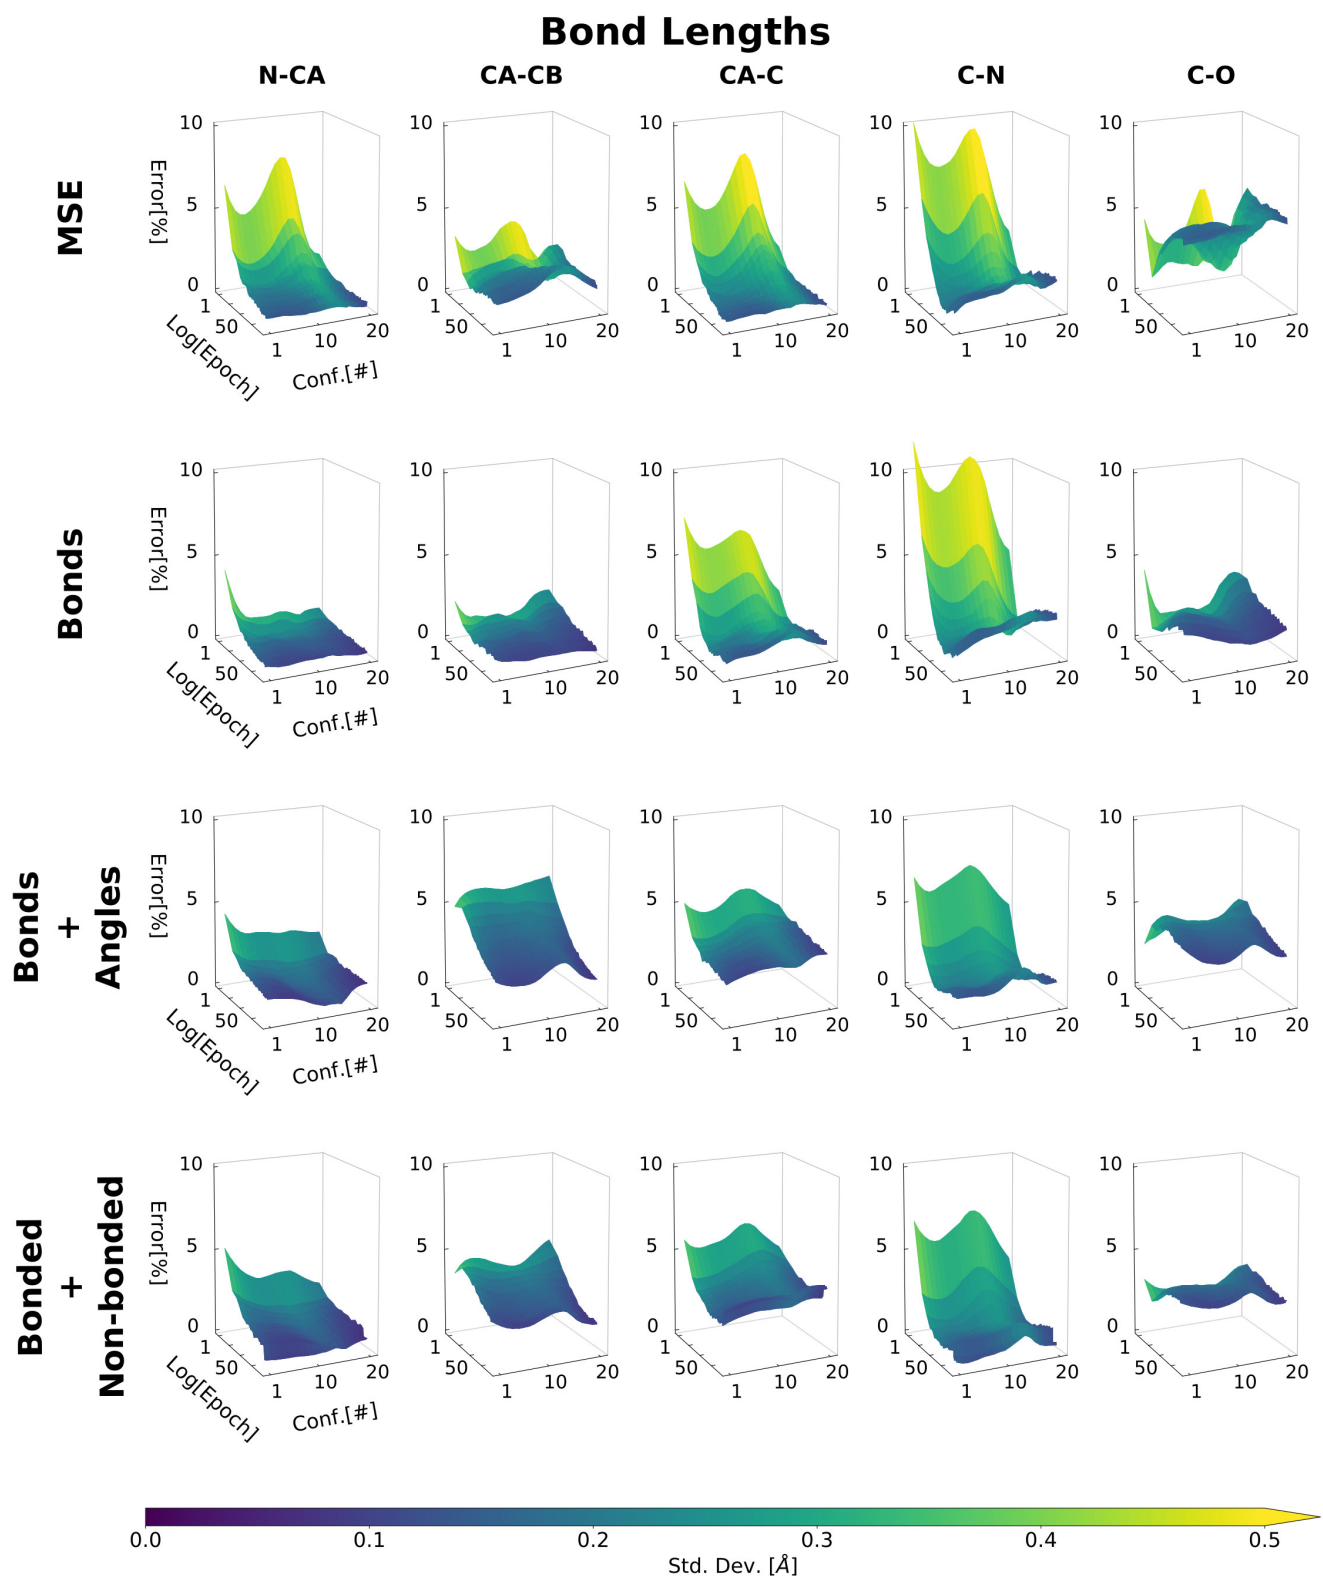

Figure S 1: Total error on interpolated structures throughout network training with different loss functions (see Main Text), decomposed by bond type. Addition of physics-based terms in the loss function improves interpolated structures quality.

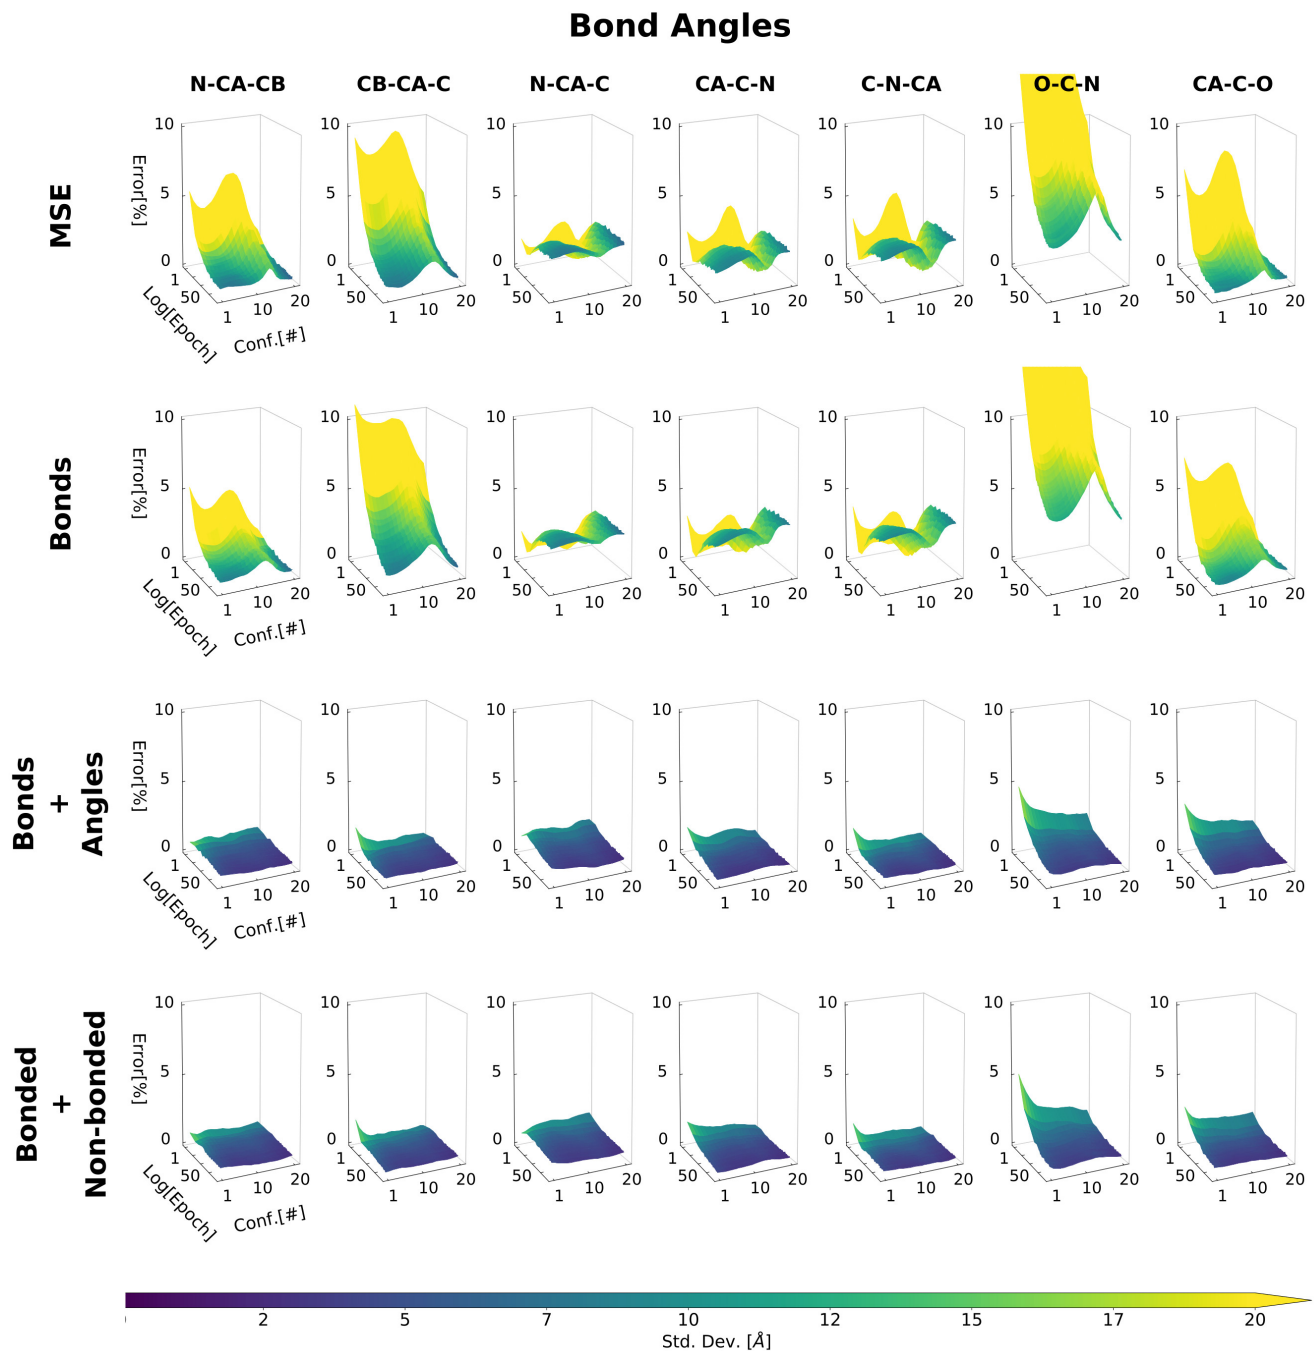

Figure S 2: Total error on interpolated structures throughout network training with different loss functions (see Main Text), decomposed by angle type. Addition of physics-based terms in the loss function improves interpolated structures quality.

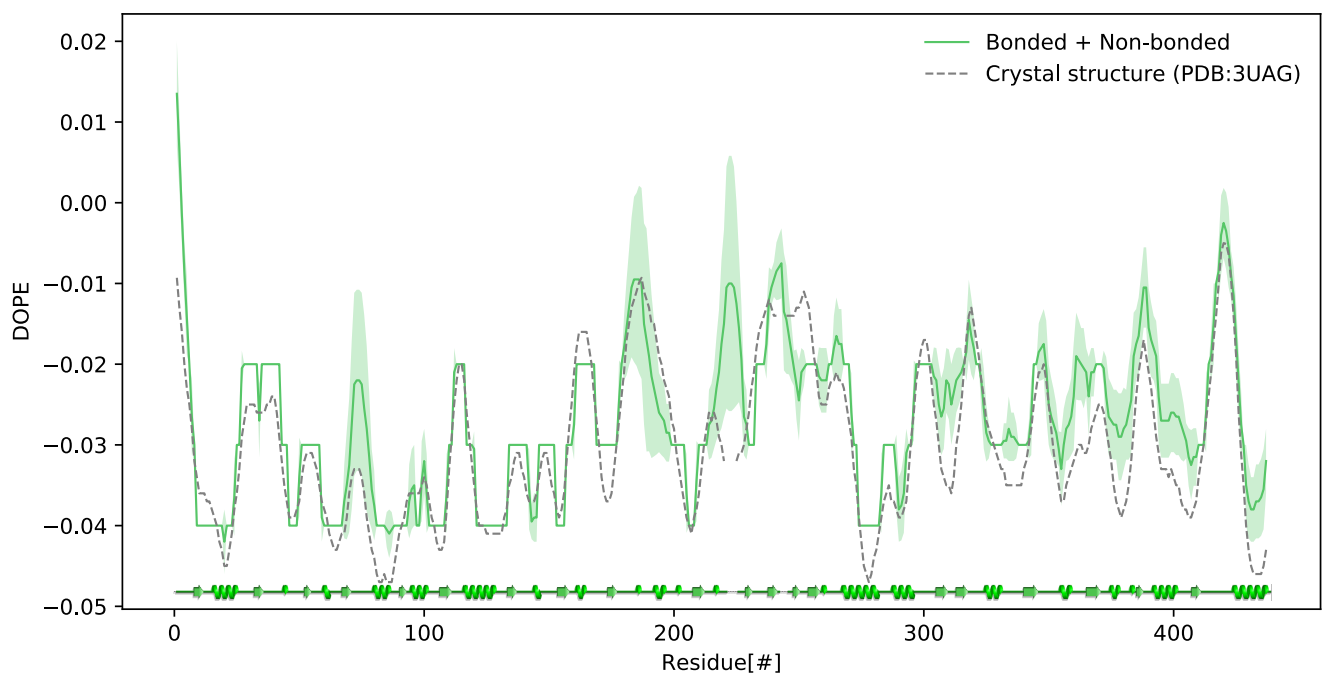

Figure S 3: DOPE score profile of the conformations generated by the best network. The mean DOPE score is plotted in bold and the corresponding standard deviations (calculated using the 20 transition state conformations) in transparent. The dashed grey line represents the DOPE profile of the MurD crystal structure in its closed state (PDB: 3UAG). The secondary structure of MurD is also shown in green at the bottom for reference (helix:  $\alpha$ -helix; arrow:  $\beta$ -strand; line: coil)

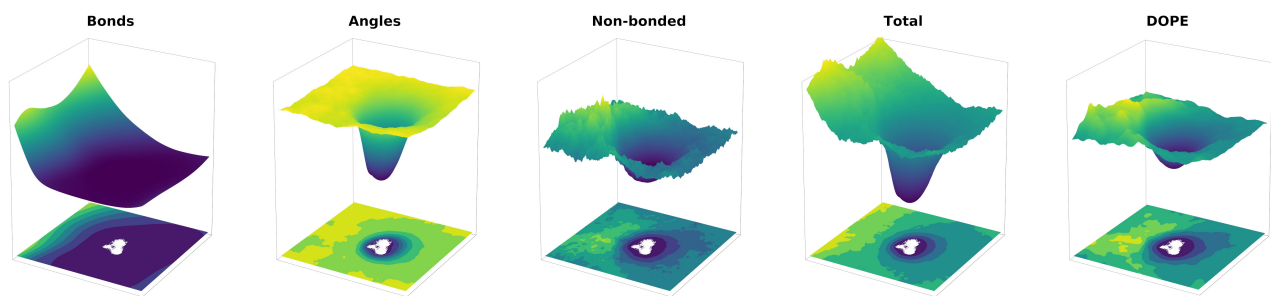

Figure S 4: Latent space landscapes of all physical loss function terms including DOPE score combine into a clearly defined minimum. White points indicate the projection in the latent space of all training examples, including the generated midpoints  $\mathbf{z}_m$ .

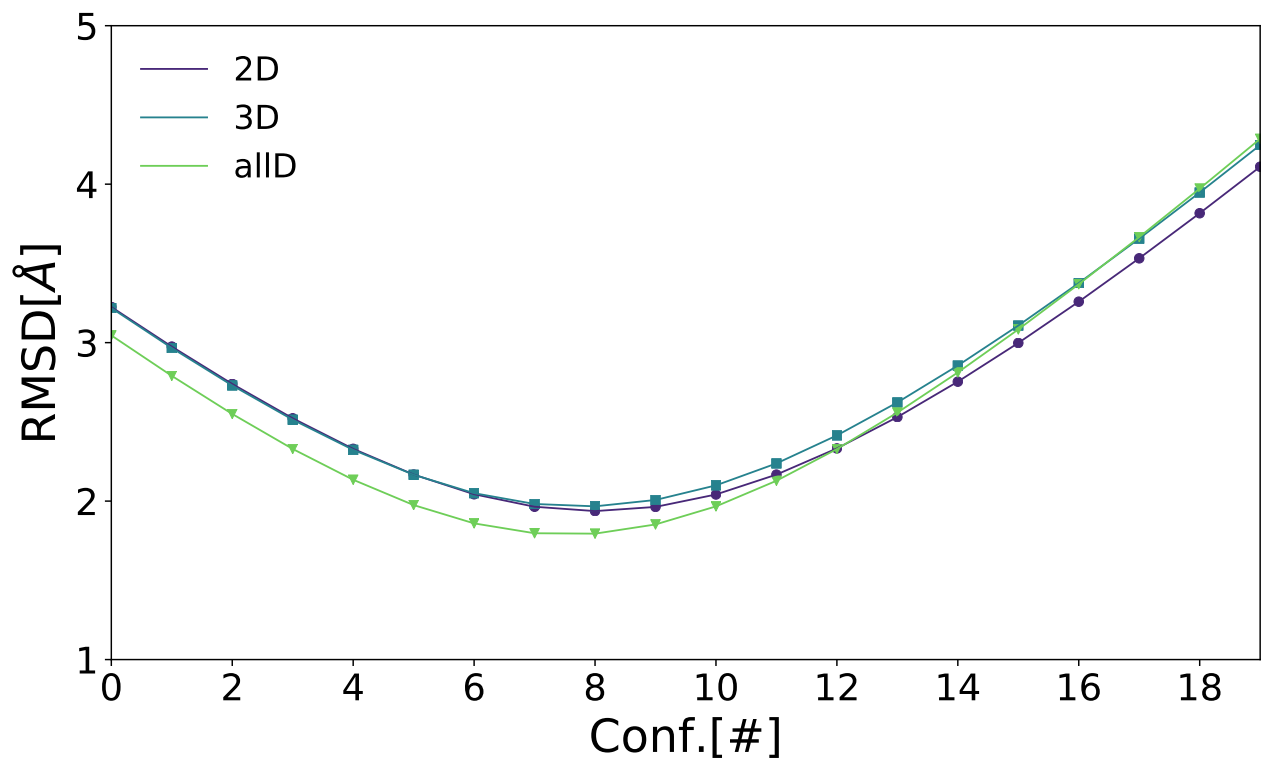

Figure S 5: Comparison of the backbone RMSD of secondary structure elements of the interpolated structures generated by PCA considering 2 dimensions (2D), 3 dimensions (3D) and all dimensions (allD) with respect to the intermediate state crystal structure (PDB: 5A5E). Increasing the number of eigenvectors describing protein motion only marginally improves the quality of the interpolated structures.

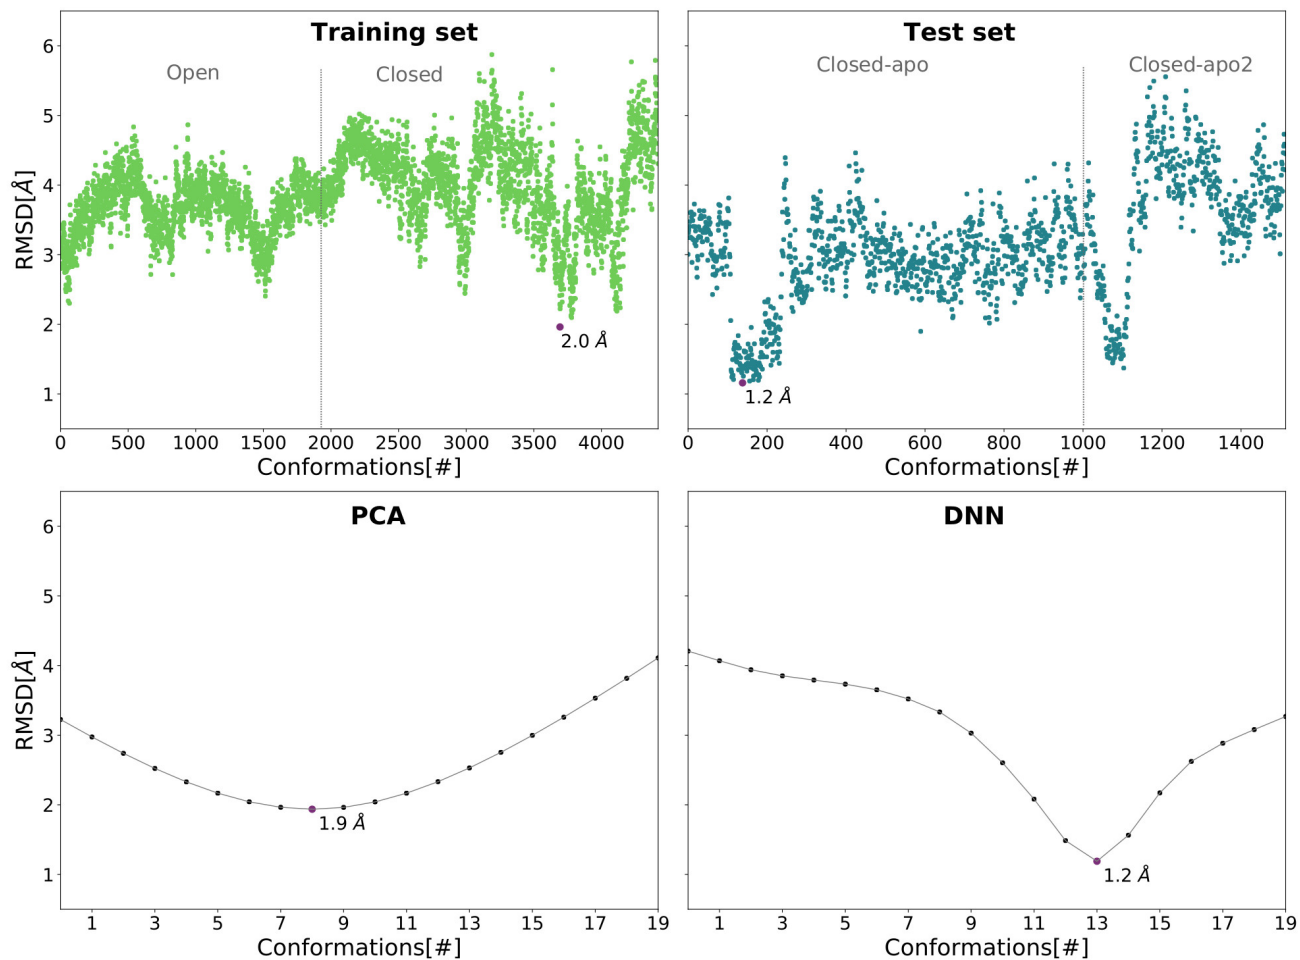

Figure S 6: Backbone RMSD of MurD structured regions with respect to the intermediate state crystal structure (PDB: 5A5E). The top panels show the RMSD of MD simulations used for training (left; open and closed states) and as test (right; closed-apo and closed-apo2). The bottom left panel reports the RMSD of structures generated via a PCA-based interpolation. The bottom right panel reports the RMSD of structures generated by interpolation of our neural network (DNN, i.e. with a loss function featuring both MSE and physics-based terms). In all images, the structure having the smallest RMSD from the intermediate MurD crystal structure 5A5E is marked with a palatinate dot. The DDN interpolation produces the model best recapitulating the intermediate MurD conformation.

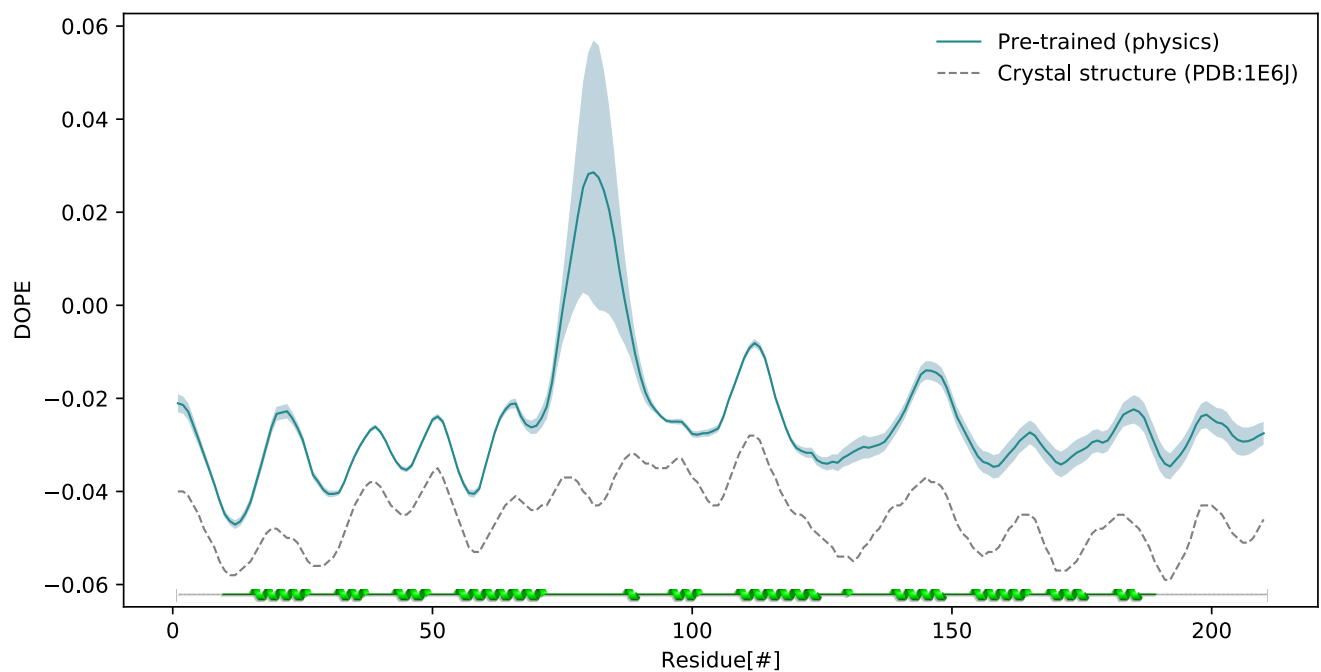

Figure S 7: Comparison of the DOPE score profile of the p24 conformations generated by the pre-trained network. The mean DOPE score is plotted in bold and the corresponding standard deviations (calculated using the 20 transition state conformations) in transparent. The dashed grey line represents the DOPE profile of the p24 crystal structure (PDB: 1E6J). The secondary structure of the protein is also shown in green at the bottom for reference (helix:  $\alpha$ -helix; line: coil). The only protein region with an invalid positive score is associated to a long, flexible loop region.

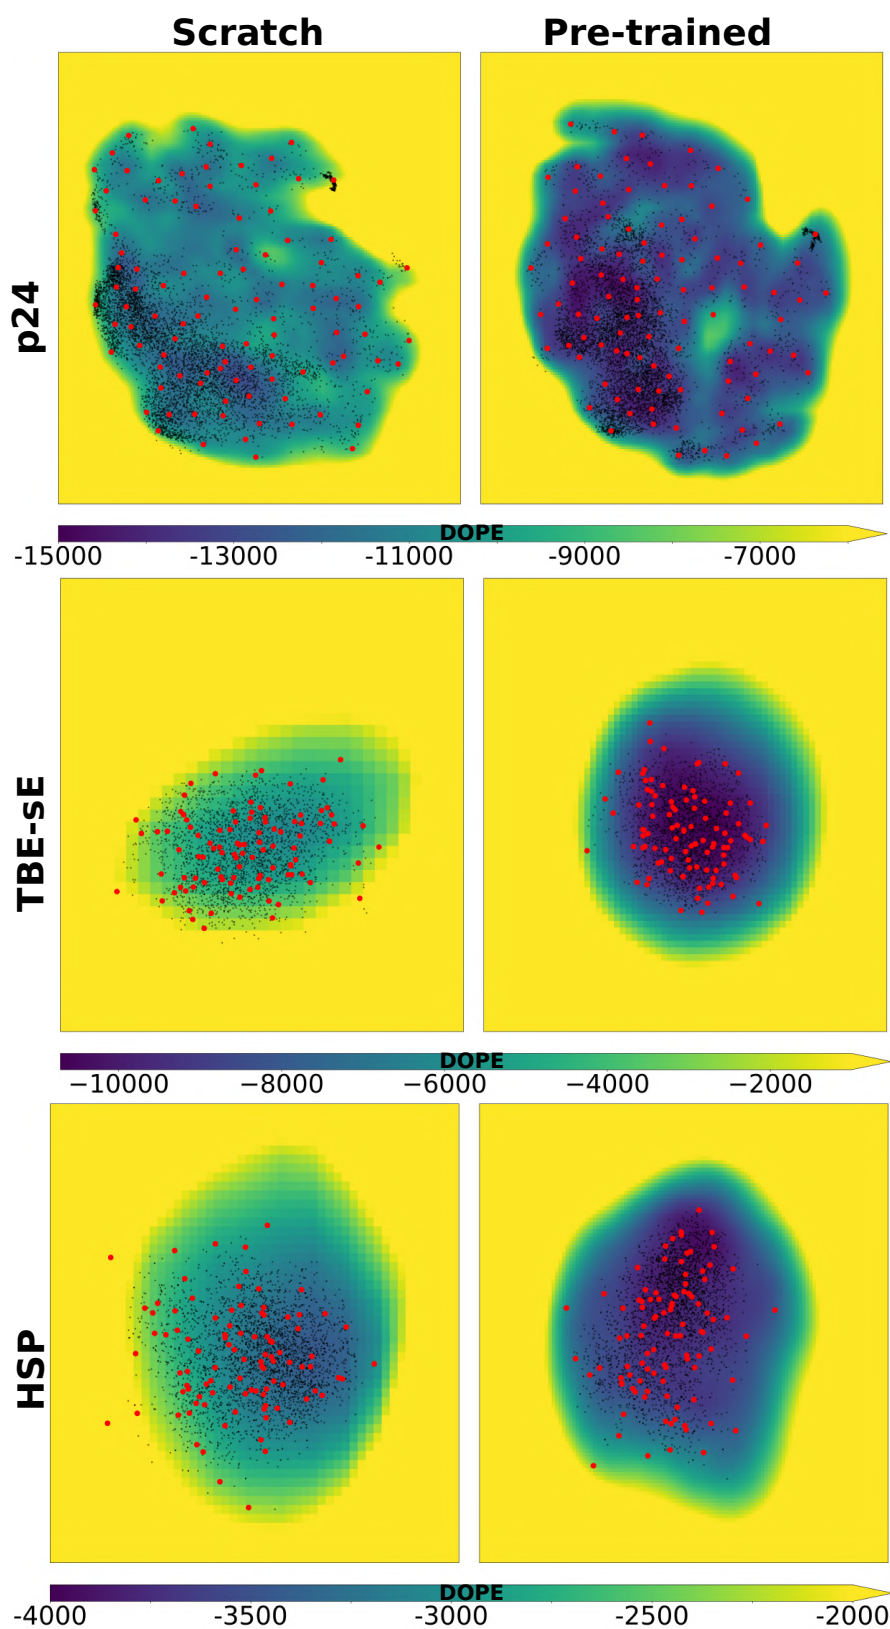

Figure S 8: Comparison of latent space DOPE scores for three proteins (p24, TBE-sE and HSP), comparing network trained from scratch or pre-trained with MurD. Black points indicate the position of all conformations obtained via MD simulation, while red points indicate the subset of 100 conformations randomly selected to be part of the training set. In all cases, the network trained by transfer learning features lower DOPE scores.

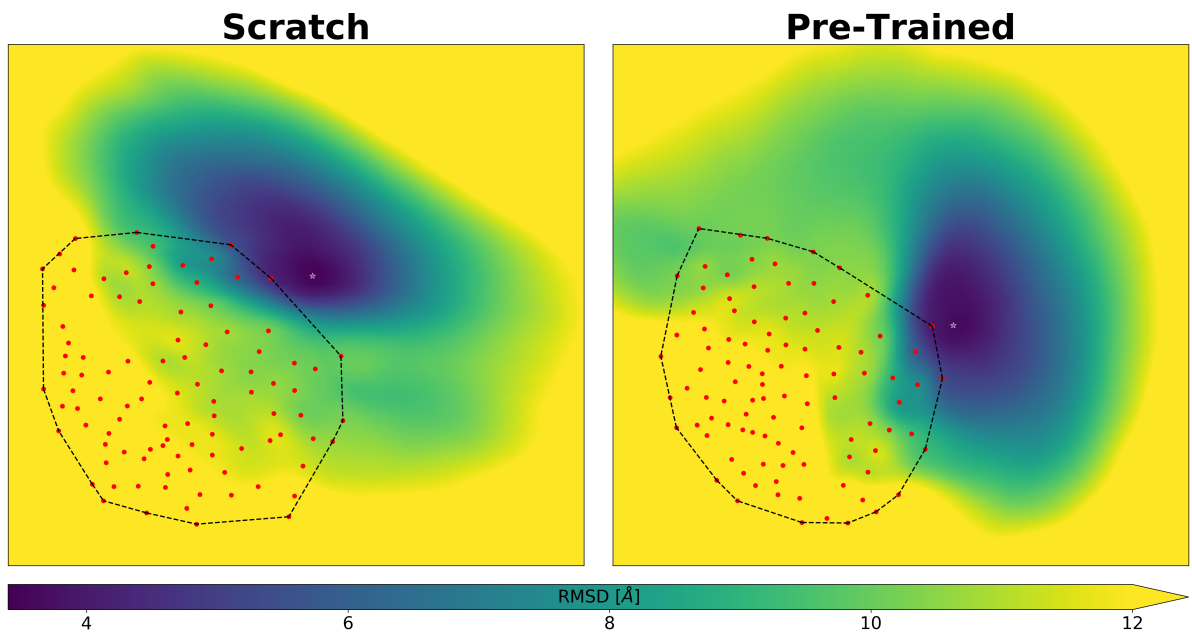

Figure S 9: Latent spaces of neural networks trained from scratch (left) and via transfer learning (right) with p24 conformations. Red points indicate the position of the 100 training set conformations, and the dashed black line shows their convex hull. The background colour indicates the local RMSD between the decoded structure and the known bound state (PDB: 3MGE), where the position of lowest value is indicated with a palatinate star. In both trained networks, the conformation with lowest RMSD from the known bound state falls outside of the training set's convex hull. In the training set, the lowest RMSD from the bound state is 4 Å, in the network trained from scratch it is 3.5 Å and in the network having parameters initialized by transfer learning it is 3.6 Å.

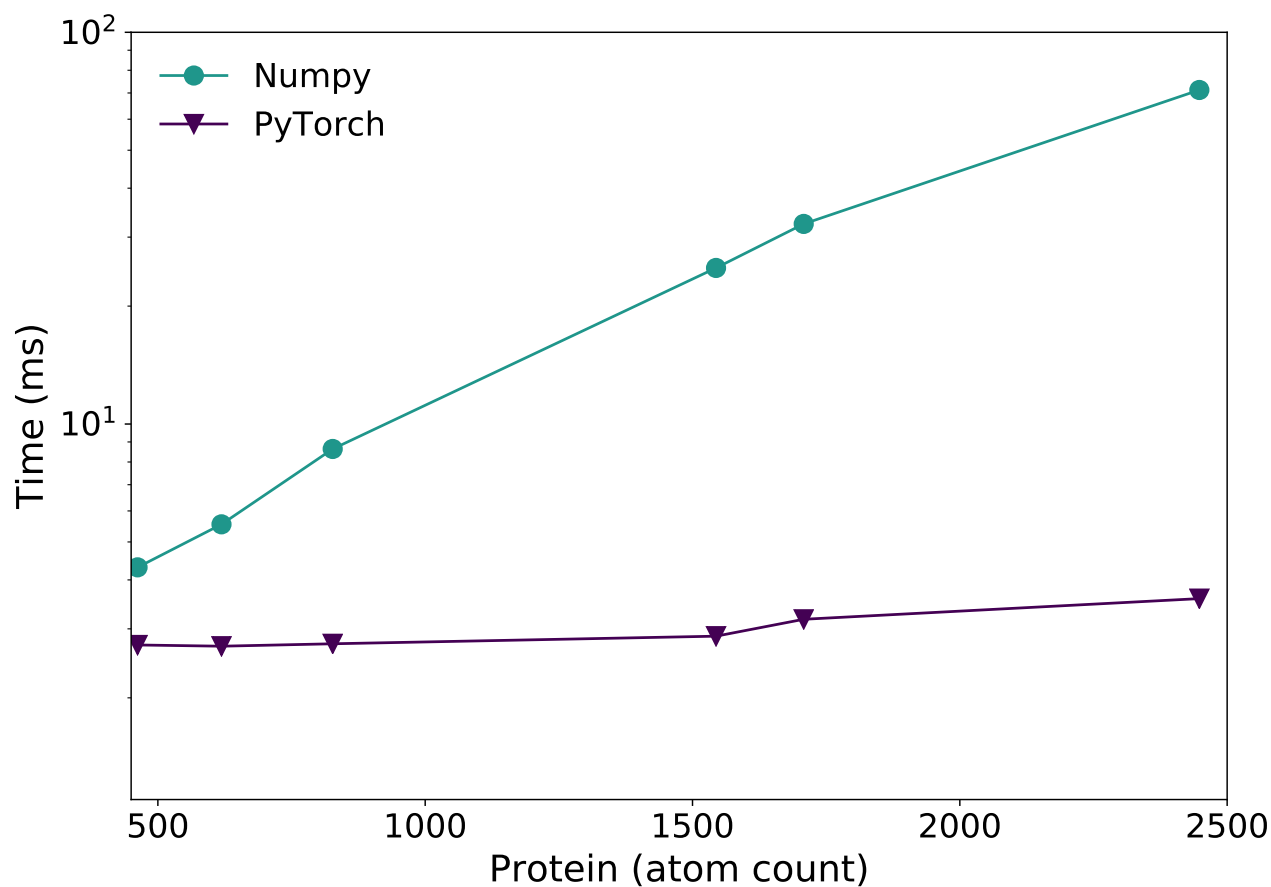

Figure S 10: Comparison of execution times (in ms) of loss functions implemented in numpy and PyTorch, evaluating physics-based terms for proteins of different sizes. The GPU PyTorch implementation running on a GTX 1080 Ti, featuring convolution-based evaluations, is more than 20 times faster.

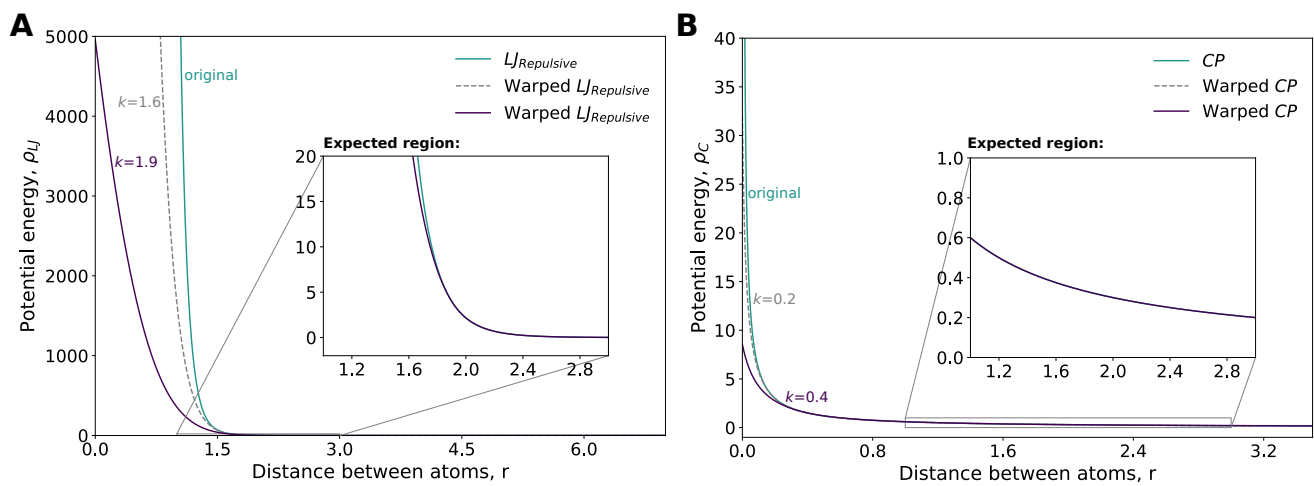

Figure S 11: Comparison of original and warped non-bonded potentials. (A) Lennard-Jones and (B) Coulomb (with charge  $q = 0.6$ )
